# Supplementary material for: Search results diversification in competitive search
Source: arXiv:2501.14922 source file (2025-01-24)
Supplement: Supplementary file 1 [file appendix.tex]

\appendix

\section{Dataset}\label{appendix_experimental_design}

\myparagraph{Initial documents} \label{appendix_queries_init_doc}
As mentioned, for each query we provided an initial relevant documen. For five queries, the initial documents were selected from a previous dataset \cite{goren_driving_2021}. To generate initial documents for an additional ten queries, we used the following procedure following Raifer \cite{raifer_information_2017}: first, we used the query in a commercial search engine and selected a highly ranked page. From this page, we extracted a candidate paragraph of up to 150 words. Three annotators then judged the relevance of the passages. We repeated the extraction process for each query until a paragraph was judged relevant by at least two annotators. The selected paragraph was then used as the initial document for the query for all students.
